# Supplementary material for: Resonant suppression of the above-barrier fusion cross-section in $^{19}$O + $^{12}$C
Source: arXiv:2501.12995 source file (2025-01-22)
Supplement: Supplementary file 1 [file Supplementary_material_Desilets.pdf]

# Supplementary Material: Resonant suppression of the above-barrier fusion cross-section in $^{19}\text{O} + ^{12}\text{C}$

H. Desilets, Rohit Kumar, R. T. deSouza, S. Hudan, C. Ciampi, A. Chbihi, K. W. Brown, K. Godbey, B. Pinheiro, E. N. Cardozo, and J. Lubian

Tabulated fusion cross-sections measured with MuSIC@Indiana during experiment E831 at GANIL. The energy error bars result from the finite width of the anode and the gas pressure inside the detector. The error bars presented in  $\sigma_F$  reflect both the statistical and systematic uncertainties of the measurement.

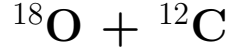

| $E_{\text{c.m.}}$ (MeV) | $N_{\text{ER}}$ (counts) | $\sigma_F$ (mb)   |
|-------------------------|--------------------------|-------------------|
| $13.03 \pm 0.35$        | 397                      | $806.7 \pm 57.4$  |
| $13.72 \pm 0.35$        | 363                      | $737.6 \pm 53.7$  |
| $14.40 \pm 0.33$        | 446                      | $906.2 \pm 62.7$  |
| $15.04 \pm 0.32$        | 415                      | $843.2 \pm 59.3$  |
| $15.69 \pm 0.33$        | 490                      | $995.6 \pm 67.4$  |
| $16.33 \pm 0.32$        | 452                      | $918.4 \pm 63.3$  |
| $16.96 \pm 0.31$        | 478                      | $971.2 \pm 66.1$  |
| $17.57 \pm 0.30$        | 476                      | $967.2 \pm 65.9$  |
| $18.18 \pm 0.31$        | 515                      | $1046.4 \pm 70.1$ |
| $18.78 \pm 0.30$        | 486                      | $987.5 \pm 67.0$  |
| $19.37 \pm 0.29$        | 611                      | $1241.5 \pm 80.3$ |
| $19.95 \pm 0.29$        | 562                      | $1141.9 \pm 75.1$ |
| $20.52 \pm 0.28$        | 540                      | $1097.2 \pm 72.7$ |

Table 1:  $^{18}\text{O} + ^{12}\text{C}$  cross-sections measured by MuSIC@Indiana. The pressure of  $\text{CH}_4$  was 150 torr.

$$^{19}\text{O} + ^{12}\text{C}$$

| $E_{\text{c.m.}}$ (MeV) | $N_{\text{ER}}$ (counts) | $\sigma_F$ (mb)  |
|-------------------------|--------------------------|------------------|
| $7.29 \pm 0.38$         | 7                        | $44.6 \pm 17.0$  |
| $8.02 \pm 0.36$         | 33                       | $210.3 \pm 38.1$ |
| $8.73 \pm 0.35$         | 60                       | $382.4 \pm 53.0$ |
| $9.42 \pm 0.33$         | 68                       | $433.4 \pm 56.9$ |
| $10.07 \pm 0.32$        | 90                       | $573.6 \pm 67.0$ |
| $10.72 \pm 0.33$        | 97                       | $618.2 \pm 70.1$ |
| $11.36 \pm 0.31$        | 94                       | $599.1 \pm 68.8$ |
| $11.99 \pm 0.31$        | 76                       | $484.4 \pm 60.7$ |
| $12.60 \pm 0.30$        | 112                      | $713.9 \pm 76.5$ |
| $13.19 \pm 0.30$        | 110                      | $701.1 \pm 75.6$ |
| $13.78 \pm 0.29$        | 125                      | $796.7 \pm 81.8$ |
| $14.36 \pm 0.28$        | 137                      | $873.2 \pm 86.6$ |
| $14.93 \pm 0.29$        | 139                      | $885.9 \pm 87.4$ |

Table 2:  $^{19}\text{O} + ^{12}\text{C}$  cross-sections measured by MuSIC@Indiana. The pressure of  $\text{CH}_4$  was 130 torr.

$$^{19}\text{F} + ^{12}\text{C}$$

| $E_{\text{c.m.}}$ (MeV) | $N_{\text{ER}}$ (counts) | $\sigma_F$ (mb)  | $E_{\text{c.m.}}$ (MeV) | $N_{\text{ER}}$ (counts) | $\sigma_F$ (mb)  |
|-------------------------|--------------------------|------------------|-------------------------|--------------------------|------------------|
| $6.34 \pm 0.55$         | 1                        | $0.4 \pm 0.4$    | $11.88 \pm 0.48$        | 1619                     | $504.0 \pm 28.3$ |
| $6.96 \pm 0.44$         | 5                        | $11.2 \pm 5.0$   | $12.03 \pm 0.43$        | 1390                     | $524.8 \pm 30.0$ |
| $7.41 \pm 0.52$         | 26                       | $9.8 \pm 2.0$    | $12.49 \pm 0.35$        | 1241                     | $580.4 \pm 33.6$ |
| $7.61 \pm 0.58$         | 58                       | $18.1 \pm 2.5$   | $12.55 \pm 0.36$        | 252                      | $564.8 \pm 45.6$ |
| $7.84 \pm 0.44$         | 14                       | $31.4 \pm 8.5$   | $12.84 \pm 0.48$        | 1978                     | $615.7 \pm 34.0$ |
| $8.42 \pm 0.48$         | 186                      | $70.2 \pm 6.2$   | $12.88 \pm 0.41$        | 1669                     | $630.1 \pm 35.3$ |
| $8.70 \pm 0.42$         | 41                       | $91.9 \pm 15.1$  | $13.18 \pm 0.34$        | 1454                     | $680.0 \pm 38.6$ |
| $8.74 \pm 0.54$         | 279                      | $86.8 \pm 6.8$   | $13.27 \pm 0.36$        | 293                      | $656.7 \pm 50.7$ |
| $8.76 \pm 0.40$         | 204                      | $95.4 \pm 8.2$   | $13.70 \pm 0.41$        | 1840                     | $694.7 \pm 38.6$ |
| $9.37 \pm 0.47$         | 601                      | $226.9 \pm 14.7$ | $13.78 \pm 0.46$        | 2261                     | $703.8 \pm 38.4$ |
| $9.52 \pm 0.40$         | 96                       | $215.2 \pm 24.5$ | $13.85 \pm 0.33$        | 1424                     | $666.0 \pm 37.9$ |
| $9.56 \pm 0.39$         | 496                      | $232.0 \pm 15.7$ | $14.49 \pm 0.39$        | 2026                     | $764.9 \pm 42.1$ |
| $9.82 \pm 0.54$         | 775                      | $241.2 \pm 14.9$ | $14.51 \pm 0.33$        | 1729                     | $808.7 \pm 45.2$ |
| $10.29 \pm 0.45$        | 873                      | $329.6 \pm 20.0$ | $14.70 \pm 0.45$        | 2376                     | $739.6 \pm 40.3$ |
| $10.32 \pm 0.39$        | 146                      | $327.2 \pm 31.7$ | $15.17 \pm 0.32$        | 1758                     | $822.2 \pm 45.9$ |
| $10.32 \pm 0.38$        | 786                      | $367.6 \pm 22.7$ | $15.28 \pm 0.39$        | 2034                     | $767.9 \pm 42.3$ |
| $10.88 \pm 0.52$        | 972                      | $302.6 \pm 18.1$ | $15.59 \pm 0.44$        | 2705                     | $842.0 \pm 45.4$ |
| $11.07 \pm 0.37$        | 848                      | $396.6 \pm 24.2$ | $15.81 \pm 0.32$        | 1836                     | $858.7 \pm 47.7$ |
| $11.08 \pm 0.37$        | 190                      | $425.9 \pm 37.6$ | $16.05 \pm 0.39$        | 2417                     | $912.5 \pm 49.6$ |
| $11.17 \pm 0.43$        | 1257                     | $474.6 \pm 27.4$ | $16.44 \pm 0.31$        | 1852                     | $866.2 \pm 48.1$ |
| $11.79 \pm 0.35$        | 1263                     | $590.7 \pm 34.1$ | $17.06 \pm 0.31$        | 2086                     | $975.6 \pm 53.6$ |
| $11.82 \pm 0.37$        | 251                      | $562.6 \pm 45.4$ |                         |                          |                  |

Table 3:  $^{19}\text{F} + ^{12}\text{C}$  cross-sections measured by MuSIC@Indiana. The pressure of  $\text{CH}_4$  was 127, 130, 155, and 175 torr during the various measurements.

$$^{20}\text{O} + ^{12}\text{C}$$

| $E_{\text{c.m.}}$ (MeV) | $N_{\text{ER}}$ (counts) | $\sigma_F$ (mb)  | $E_{\text{c.m.}}$ (MeV) | $N_{\text{ER}}$ (counts) | $\sigma_F$ (mb)   |
|-------------------------|--------------------------|------------------|-------------------------|--------------------------|-------------------|
| 6.15 $\pm$ 0.34         | 30                       | 19.4 $\pm$ 3.7   | 12.94 $\pm$ 0.26        | 1022                     | 772.6 $\pm$ 45.8  |
| 6.47 $\pm$ 0.33         | 52                       | 39.3 $\pm$ 5.8   | 13.06 $\pm$ 0.25        | 1258                     | 793.0 $\pm$ 45.8  |
| 6.47 $\pm$ 0.38         | 23                       | 30.0 $\pm$ 6.4   | 13.37 $\pm$ 0.24        | 2492                     | 778.2 $\pm$ 42.2  |
| 6.82 $\pm$ 0.33         | 90                       | 56.8 $\pm$ 6.6   | 13.45 $\pm$ 0.28        | 692                      | 903.7 $\pm$ 57.1  |
| 7.13 $\pm$ 0.33         | 80                       | 60.5 $\pm$ 7.4   | 13.45 $\pm$ 0.26        | 1161                     | 877.7 $\pm$ 51.2  |
| 7.21 $\pm$ 0.35         | 54                       | 70.5 $\pm$ 10.2  | 13.56 $\pm$ 0.25        | 1448                     | 913.2 $\pm$ 51.9  |
| 7.45 $\pm$ 0.30         | 169                      | 106.6 $\pm$ 9.8  | 13.85 $\pm$ 0.23        | 2671                     | 833.8 $\pm$ 45.0  |
| 7.77 $\pm$ 0.32         | 236                      | 178.4 $\pm$ 14.7 | 13.95 $\pm$ 0.25        | 1906                     | 829.0 $\pm$ 45.9  |
| 7.90 $\pm$ 0.34         | 143                      | 186.8 $\pm$ 18.2 | 13.97 $\pm$ 0.26        | 1197                     | 904.9 $\pm$ 52.6  |
| 8.06 $\pm$ 0.31         | 388                      | 244.7 $\pm$ 17.5 | 14.01 $\pm$ 0.28        | 679                      | 886.7 $\pm$ 56.2  |
| 8.40 $\pm$ 0.31         | 353                      | 266.9 $\pm$ 19.6 | 14.06 $\pm$ 0.25        | 1357                     | 859.4 $\pm$ 49.2  |
| 8.56 $\pm$ 0.33         | 225                      | 293.8 $\pm$ 24.6 | 14.18 $\pm$ 0.26        | 1486                     | 850.8 $\pm$ 48.2  |
| 8.67 $\pm$ 0.30         | 474                      | 301.1 $\pm$ 20.5 | 14.33 $\pm$ 0.24        | 2692                     | 839.6 $\pm$ 45.3  |
| 9.01 $\pm$ 0.31         | 537                      | 406.0 $\pm$ 26.9 | 14.46 $\pm$ 0.26        | 1961                     | 852.9 $\pm$ 47.1  |
| 9.23 $\pm$ 0.33         | 366                      | 478.0 $\pm$ 34.7 | 14.48 $\pm$ 0.25        | 1098                     | 830.1 $\pm$ 48.8  |
| 9.26 $\pm$ 0.30         | 733                      | 462.1 $\pm$ 28.9 | 14.56 $\pm$ 0.25        | 1353                     | 854.5 $\pm$ 49.0  |
| 9.62 $\pm$ 0.29         | 601                      | 454.4 $\pm$ 29.5 | 14.71 $\pm$ 0.26        | 1565                     | 896.1 $\pm$ 50.5  |
| 9.85 $\pm$ 0.29         | 796                      | 502.7 $\pm$ 31.0 | 14.80 $\pm$ 0.23        | 2967                     | 925.3 $\pm$ 49.6  |
| 9.88 $\pm$ 0.32         | 370                      | 483.2 $\pm$ 35.0 | 14.96 $\pm$ 0.24        | 2114                     | 919.4 $\pm$ 50.5  |
| 10.20 $\pm$ 0.29        | 782                      | 591.2 $\pm$ 36.5 | 15.23 $\pm$ 0.26        | 1653                     | 946.4 $\pm$ 53.1  |
| 10.41 $\pm$ 0.28        | 935                      | 590.1 $\pm$ 35.5 | 15.26 $\pm$ 0.23        | 2935                     | 915.5 $\pm$ 49.2  |
| 10.51 $\pm$ 0.31        | 448                      | 585.1 $\pm$ 40.4 | 15.44 $\pm$ 0.25        | 2154                     | 936.8 $\pm$ 51.4  |
| 10.77 $\pm$ 0.29        | 751                      | 567.8 $\pm$ 35.3 | 15.72 $\pm$ 0.23        | 3202                     | 999.0 $\pm$ 53.4  |
| 10.96 $\pm$ 0.27        | 864                      | 544.8 $\pm$ 33.1 | 15.75 $\pm$ 0.25        | 1687                     | 965.9 $\pm$ 54.1  |
| 11.12 $\pm$ 0.30        | 536                      | 700.0 $\pm$ 46.5 | 15.93 $\pm$ 0.24        | 2162                     | 940.3 $\pm$ 51.5  |
| 11.33 $\pm$ 0.27        | 907                      | 685.7 $\pm$ 41.4 | 16.18 $\pm$ 0.22        | 3183                     | 993.0 $\pm$ 53.1  |
| 11.50 $\pm$ 0.27        | 1207                     | 762.0 $\pm$ 44.2 | 16.25 $\pm$ 0.25        | 1833                     | 1049.5 $\pm$ 58.3 |
| 11.72 $\pm$ 0.30        | 592                      | 773.1 $\pm$ 50.3 | 16.42 $\pm$ 0.24        | 2482                     | 1079.5 $\pm$ 58.6 |
| 11.87 $\pm$ 0.27        | 1018                     | 769.6 $\pm$ 45.7 | 16.63 $\pm$ 0.22        | 3529                     | 1100.9 $\pm$ 58.5 |
| 12.03 $\pm$ 0.27        | 1209                     | 762.1 $\pm$ 44.2 | 16.74 $\pm$ 0.25        | 1788                     | 1023.7 $\pm$ 57.0 |
| 12.31 $\pm$ 0.29        | 602                      | 786.2 $\pm$ 51.0 | 16.89 $\pm$ 0.23        | 2373                     | 1032.1 $\pm$ 56.2 |
| 12.41 $\pm$ 0.27        | 1043                     | 788.5 $\pm$ 46.7 | 17.07 $\pm$ 0.22        | 3258                     | 1016.5 $\pm$ 54.3 |
| 12.55 $\pm$ 0.26        | 1384                     | 872.4 $\pm$ 49.8 | 17.24 $\pm$ 0.24        | 1815                     | 1039.2 $\pm$ 57.8 |
| 12.88 $\pm$ 0.25        | 2646                     | 825.2 $\pm$ 44.6 | 17.36 $\pm$ 0.24        | 2353                     | 1023.4 $\pm$ 55.7 |
| 12.89 $\pm$ 0.28        | 701                      | 915.5 $\pm$ 57.7 | 17.51 $\pm$ 0.22        | 3275                     | 1021.6 $\pm$ 54.5 |

Table 4:  $^{20}\text{O} + ^{12}\text{C}$  cross-sections measured by MuSIC@Indiana. The pressure of  $\text{CH}_4$  was 110, 115, 117, 118, 124, and 130 torr during the various measurements.
